# Supplementary material for: JUMP: Efficient Membership Inference on Fine-Tuned Diffusion Language Models
Source: arXiv:2607.16207 source file (2026-09-28)
Supplement: Supplementary file 1 [file limitations.tex]

\label[appendix]{app:limitation}

Our experiments focus on membership inference for fine-tuned dLLMs, where membership is defined with respect to the fine-tuning set.
This setting isolates the effect of the dLLM masking interface and avoids the additional ambiguity of pretraining-scale membership, where exposure, deduplication, and near-duplicate examples are difficult to control.
Extending the analysis to pretraining-scale dLLMs is an important direction for future work.

JUMP uses a reference model to calibrate example difficulty, following the common practice of reference-based MIAs.
In our main experiments, the reference model is the pretrained checkpoint before fine-tuning, which provides a clean way to measure the effect of fine-tuning.
We note, however, that the attack does not rely on target-model internals, and the selector itself is trained only on generic public text without member labels or target weights.
Moreover, our PRISM-Free variant removes auxiliary selector training and still remains competitive, suggesting that the core single-pass probing idea is not tied to a specific learned selector.

Finally, our evaluation covers two recent dLLM families, with LLaDA as the main model and Dream as a secondary-model check.
The relative strength of JUMP and SAMA can vary across model families, but the experiments consistently show that joint masked probing provides a strong dLLM-specific membership signal.
We therefore view JUMP as a first single-pass baseline for fine-tuned dLLM MIA, and broader evaluation across future dLLM architectures as natural follow-up work.
