# Supplementary material for: JUMP: Efficient Membership Inference on Fine-Tuned Diffusion Language Models
Source: arXiv:2607.16207 source file (2026-09-28)
Supplement: Supplementary file 2 [file prism_free.tex]

\subsection{PRISM-Free per-domain results}
\label[appendix]{app:prism_free}

\begin{table}[t]
\centering
\small
\caption{PRISM-Free per-domain results. Compare with SAMA and \method{} in \cref{tab:main_results}.}
\label{tab:app_prism_free}
\begin{tabular}{lcccc}
\toprule
Domain & AUC & TPR@10\% & TPR@1\% & TPR@0.1\% \\
\midrule
ArXiv      & 0.890 & 0.671 & 0.322 & 0.121 \\
GitHub     & 0.859 & 0.650 & 0.222 & 0.128 \\
HackerNews & 0.758 & 0.361 & 0.069 & 0.010 \\
Pile-CC    & 0.940 & 0.828 & 0.510 & 0.175 \\
PubMed     & 0.817 & 0.535 & 0.166 & 0.011 \\
Wikipedia  & 0.958 & 0.887 & 0.631 & 0.362 \\
\midrule
Mean       & 0.870 & 0.655 & 0.320 & 0.135 \\
\bottomrule
\end{tabular}
\end{table}
